# Supplementary material for: Mobile IMUs Reveal Driver's Identity From Vehicle Turns
Source: arXiv:1710.04578 source file (2017-10-12)
Supplement: Supplementary file 1 [file appendix.tex]

\appendix
\section{This Sec 1 of App}

\dc{
In the data collection process, {\name} stores IMU data in JSON file formate and compress the data before uploading to cloud. According to our experiment results, {\name} only generates less than 3MB data per hour. As we will show in Sec.~\ref{subsec:overhead}, our data collection scheme minimizes energy overhead caused by {\name}.
}
\dc{
Also notice to further minimize energy overhead in real-life, an adversary can restrict {\name} to upload data only if the mobile device has WiFi connection~\cite{energy_overhead_paper}.
}
